# Supplementary material for: Sim911: Towards Effective and Equitable 9-1-1 Dispatcher Training with an LLM-Enabled Simulation
Source: arXiv:2412.16844 source file (2024-12-26)
Supplement: Supplementary file 1 [file _supplementary.tex]

\newpage
\clearpage
\newpage
% https://aaai.org/aaai-conference/reproducibility-checklist/
\section*{Reproducibility Checklist}
This paper
\begin{itemize}
    \item Includes a conceptual outline and/or pseudocode description of AI methods introduced \textbf{yes}
    \item Clearly delineates statements that are opinions, hypothesis, and speculation from objective facts and results \textbf{yes}
    \item Provides well marked pedagogical references for less-familiare readers to gain background necessary to replicate the paper \textbf{yes}
\end{itemize}
Does this paper make theoretical contributions? \textbf{yes}
If yes, please complete the list below.
\begin{itemize}
    \item All assumptions and restrictions are stated clearly and formally. \textbf{yes}
    \item All novel claims are stated formally (e.g., in theorem statements). \textbf{yes}
    \item Proofs of all novel claims are included. \textbf{yes}
    \item Proof sketches or intuitions are given for complex and/or novel results. \textbf{yes}
    \item Appropriate citations to theoretical tools used are given. \textbf{yes}
    \item All theoretical claims are demonstrated empirically to hold. \textbf{yes}
    \item All experimental code used to eliminate or disprove claims is included. \textbf{NA}
\end{itemize}
Does this paper rely on one or more datasets? \textbf{yes}
If yes, please complete the list below.
\begin{itemize}
    \item A motivation is given for why the experiments are conducted on the selected datasets \textbf{yes}
    \item All novel datasets introduced in this paper are included in a data appendix. \textbf{yes}
    \item All novel datasets introduced in this paper will be made publicly available upon publication of the paper with a license that allows free usage for research purposes. \textbf{yes}
    \item All datasets drawn from the existing literature (potentially including authors’ own previously published work) are accompanied by appropriate citations. \textbf{yes}
    \item All datasets drawn from the existing literature (potentially including authors’ own previously published work) are publicly available. \textbf{yes}
    \item All datasets that are not publicly available are described in detail, with explanation why publicly available alternatives are not scientifically satisficing. \textbf{yes, all sensitive/private data will be eventually released after de-identification.}
\end{itemize}
Does this paper include computational experiments? (yes/no)
If yes, please complete the list below.
\begin{itemize}
    \item Any code required for pre-processing data is included in the appendix. \textbf{yes}
    \item All source code required for conducting and analyzing the experiments is included in a code appendix. \textbf{yes}
    \item All source code required for conducting and analyzing the experiments will be made publicly available upon publication of the paper with a license that allows free usage for research purposes. \textbf{yes}
    \item All source code implementing new methods have comments detailing the implementation, with references to the paper where each step comes from \textbf{yes}
    \item If an algorithm depends on randomness, then the method used for setting seeds is described in a way sufficient to allow replication of results. \textbf{yes}
    \item This paper specifies the computing infrastructure used for running experiments (hardware and software), including GPU/CPU models; amount of memory; operating system; names and versions of relevant software libraries and frameworks. \textbf{yes}
    \item This paper formally describes evaluation metrics used and explains the motivation for choosing these metrics. \textbf{yes}
    \item This paper states the number of algorithm runs used to compute each reported result. \textbf{yes}
    \item Analysis of experiments goes beyond single-dimensional summaries of performance (e.g., average; median) to include measures of variation, confidence, or other distributional information. \textbf{yes}
    \item The significance of any improvement or decrease in performance is judged using appropriate statistical tests (e.g., Wilcoxon signed-rank). \textbf{yes}
    \item This paper lists all final (hyper-)parameters used for each model/algorithm in the paper’s experiments. \textbf{yes}
    \item This paper states the number and range of values tried per (hyper-)parameter during development of the paper, along with the criterion used for selecting the final parameter setting. \textbf{yes}
\end{itemize}
